# Supplementary material for: Continual Learning in Neural Networks
Source: arXiv:1910.02718 source file (2019-10-18)
Supplement: Supplementary file 1 [file appendix.tex]

\section*{Appendix}

\section{Details on the experimental setup}
In all designed experiments, our regularizer is applied to the neurons of the fully connected layers. As a future work, we plan to integrate it in the convolutional layers.
\label{appendix:experimental-setup}
\subsection{Permuted Mnist}
The used network is composed of two fully connected layers. All tasks are trained for 10 epochs with a learning rate $10^{-2}$ using SGD optimizer. ReLU is used as an activation function unless mentioned otherwise.
Throughout the experiment, we used a scale $\sigma$ for the Gaussian function used for the local inhibition equal to $1/6$ of the hidden layer size. 
For all competing
%the studied 
regularizers, we tested different hyper parameters from $10^{-2}$ to $10^{-9}$ and report the best one. 
%$\lambda_{\Omega}$, 
For $\lambda_{\Omega}$, we have used a high $\lambda_{\Omega}$ value that ensures the least forgetting.
This allows us to examine the degradation in the performance  on the later tasks compared to those learned previously as a result of lacking capacity. Note that better average accuracies can be obtained with tuned $\lambda_{\Omega}$.

In section~\ref{sec:experiments:analysis} we estimated the free capacity in the network with the percentage of $\Omega_{k} < 10^{-2}$, with $\Omega_{k}$, 
the importance weight multiplier estimated and accumulated over tasks. We consider $\Omega_{k} < 10^{-2}$ of negligible importanc as in a network trained without a sparsity regularizer, $\Omega_{ij} < 10^{-2}$ covers the first 10 percentiles. 
\subsection{CIFAR-100}
As a base network, we use %two convolutional layers followed by one fully connected layer and then a  unique classification layer per task with softmax loss. This is
a network similar to the one used by~\cite{Zenke2017improved} but without dropout. We evaluate two variants with hidden size $N=\{256,128\}$.
Throughout the experiment, we again used a scale $\sigma$ for the Gaussian function  equal to $1/6$ of the hidden layer size. %  Two different sizes of the fully connected layer $N=\{256,128\}$ were tested. 
We train the different tasks  for 50 epochs with a learning rate of $10^{-2}$ using SGD optimizer.
\subsection{Tiny ImageNet}
 We split the Tiny ImageNet dataset~\cite{yao2015tiny} into ten tasks, each containing twenty categories to be learned at once. As a base network, we use a variant of VGG~\cite{simonyan2014very}.
 For architecture details, please refer to Table~\ref{tab:arch_imagenet} below.
 \begin{table}[h]
\centering
 \begin{tabular}{|l|l|}
\hline
Layer& \# filters/neurons\\
\hline
Convolution&64\\
Max Pooling&-\\
Convolution&128\\
Max Pooling&-\\
Convolution& 256\\
Max Pooling&-\\
Convolution& 256\\
Max Pooling&-\\
Convolution& 512\\
Convolution& 512\\
Fully connected & 500\\
Fully connected & 500\\
Fully connected & 20\\
\hline
\end{tabular}
\caption{Architecture of the network used in the Tiny Imagenet experiment.}
\label{tab:arch_imagenet}
 \end{table}

 Throughout the experiment, we again used a scale $\sigma$ for the Gaussian function equal to $1/6$ of the hidden layer size. 
 \subsection{8 task object recognition sequence}
\label{appendix:experimental-setup:objects}
 The 8 tasks sequence is composed of: 1. Oxford \textit{Flowers}~\cite{Nilsback08}, 2. MIT \textit{Scenes} \cite{quattoni2009recognizing}, 3. Caltech-UCSD \textit{Birds}~\cite{WelinderEtal2010}, 4. Stanford  {\tt Cars}~\cite{krause20133d}; 5. FGVC-{\tt Aircraft}~\cite{maji13fine-grained}; 6. VOC {\tt Actions}
%, for human  action classification
~\cite{pascal-voc-2012}; 7. {\tt Letters}~\cite{deCampos09}; and 8. {\tt SVHN}~\cite{netzer2011reading} datasets. 
We have rerun the different methods and obtain the same reported results as in ~\cite{aljundi2017memory}.

\section{Extra Results}
\label{appendix:additional}
\subsection{Permuted Mnist Sequence}
In section \ref{sec:experiments:analysis}, we have studied the performance of different regularizers and activation functions on 5 permuted Mnist tasks in a network with a hidden layer of size $128$.
Figure~\ref{fig:perm_comp_64} shows the average accuracies achieved by each of the studied methods at the end of the learned sequence in a network with a hidden layer of size $64$. Similar conclusions can be drawn. {\tt Maxout} and {\tt LWTA} perform similarly
%closely 
and improve slightly over {\tt ReLU}. Regularizers applied to the representation are more powerful for sequential learning than regularizers applied directly to the parameters. Specifically, {\tt L1-Rep} (orange) is consistently better than {L1-Param} (pink). Our \SLNI is able of maintaining a good performance on all the tasks, achieving among the top average test accuracies.  
Admittedly, the performances of \SLNI is very close to L1-Rep. The difference between these methods stands out more clearly for larger networks and more complex tasks.

\begin{figure*}[h]
\centering

\includegraphics[width=0.95\textwidth]{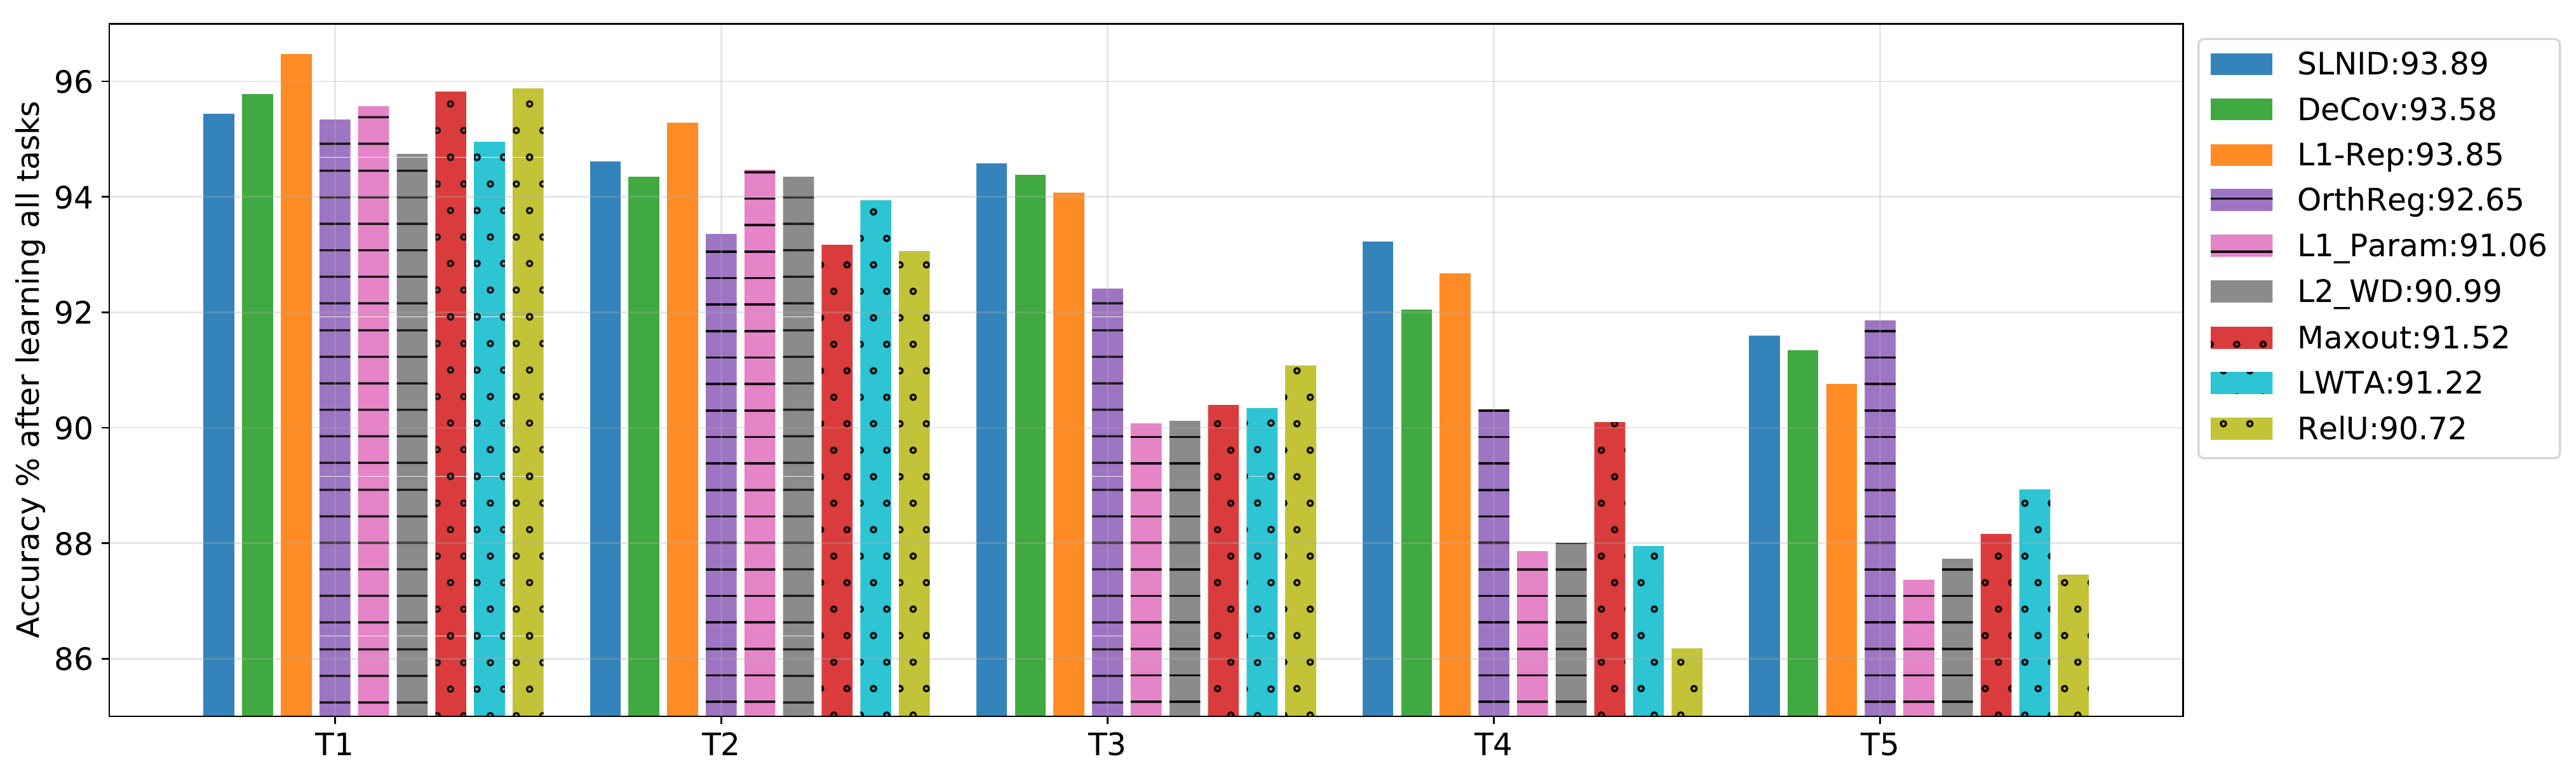} 
     \caption{\footnotesize Comparison of different regularization techniques on 5 permuted MNIST sequence of tasks, hidden size=64. Representation based regularizers are solid bars, bars with lines represent parameters regularizers, dotted bars represent activation functions. See Figure~\ref{fig:perm_comp} for size $128$.}%
    \label{fig:perm_comp_64}%

\end{figure*}
\subsection{SLNI with EWC}
To show that our approach is not limited to {\tt MAS}~\cite{aljundi2017memory}, we have also experimented with EWC~\cite{kirkpatrick2016overcoming} as another importance weight based method along with our regularize \SLNI on the permuted Mnist sequence.
Figure~\ref{fig:SLNI_EWC} shows the test accuracy of each task at the end of the 5 permuted Mnist sequence achieved by our \SLNI combined with {\tt EWC} and by {\tt No-Reg } (here indicating {\tt EWC} without regularization). It is clear that \SLNI succeeds to improve the performance on all the learned tasks which validates the utility of our approach with different sequential learning methods.
\begin{figure}[h]
\vspace*{-0.2cm}
    \centering
    \subfloat{{\includegraphics[width=0.495\textwidth]{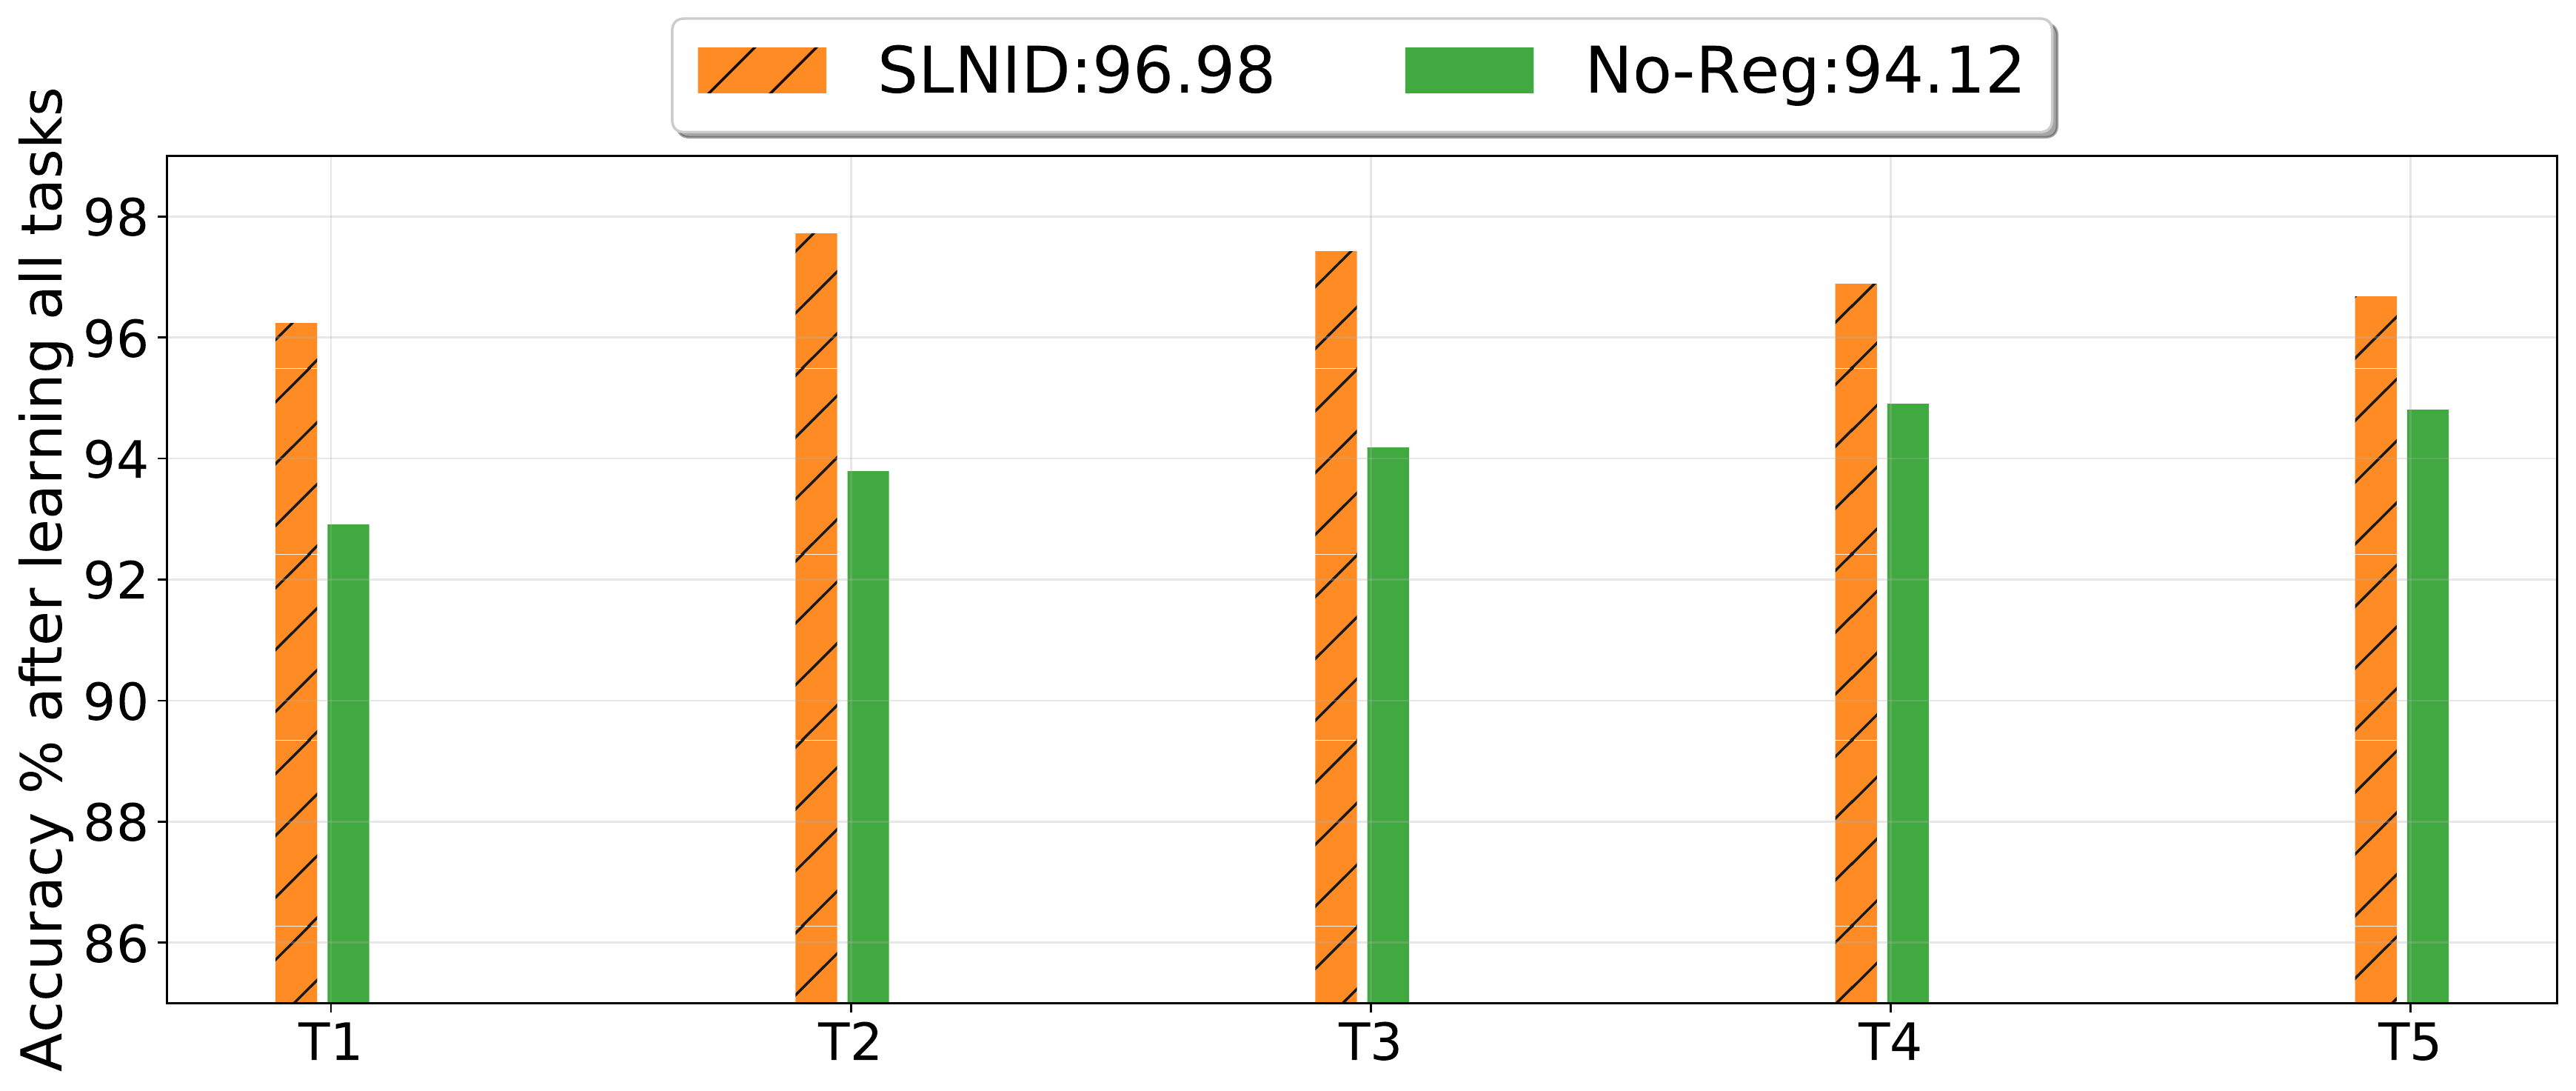} }}%
    \hfillx
    \subfloat{{\includegraphics[width=0.495\textwidth]{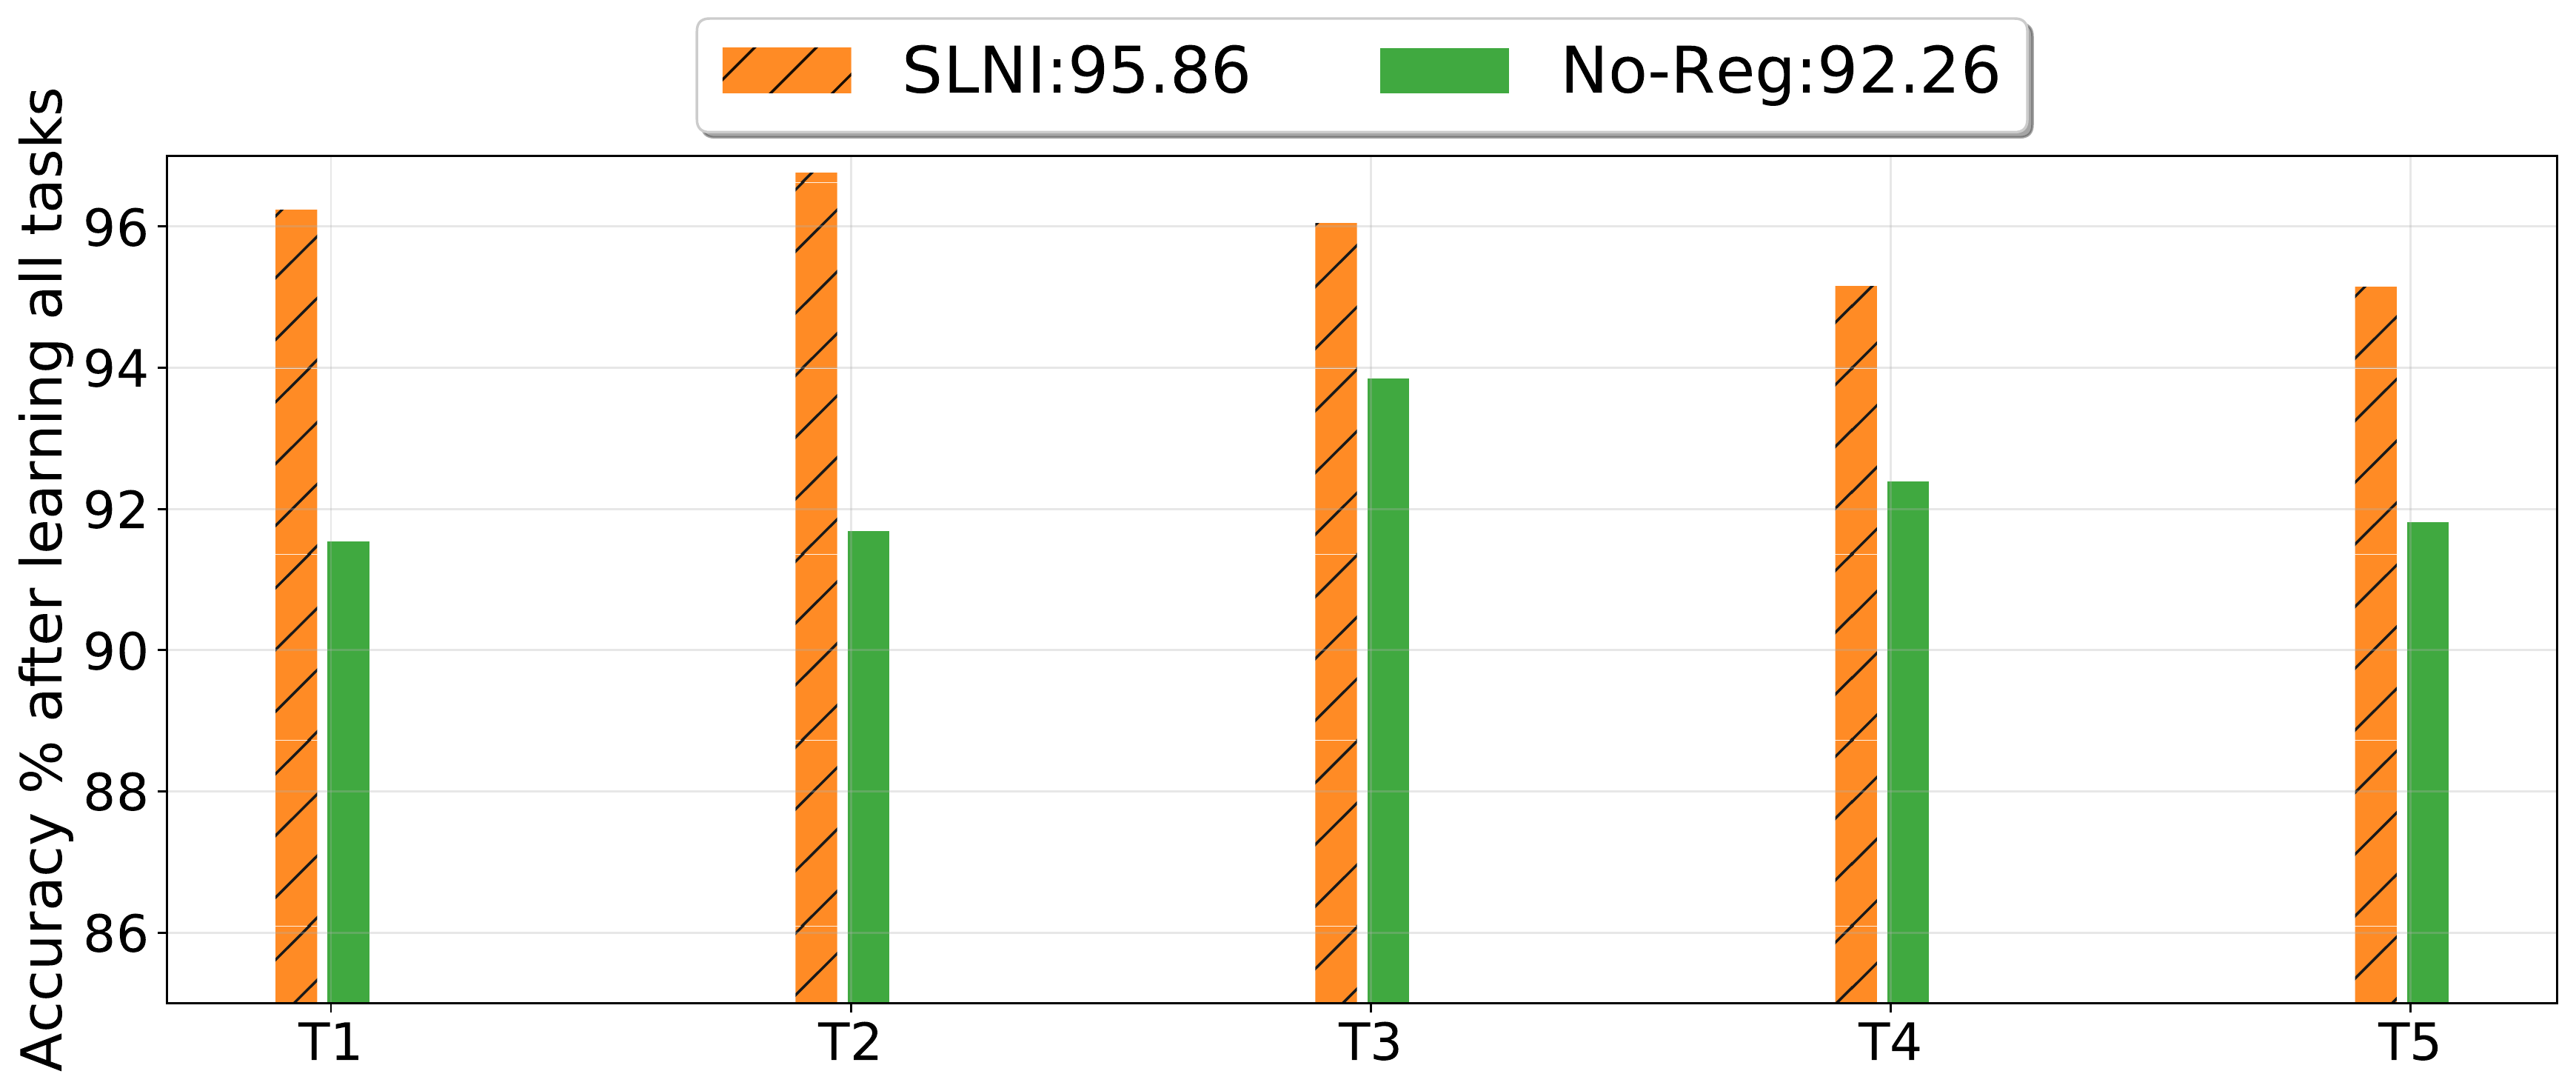} }}%
  
    \caption{\footnotesize (a) \SLNI with {\tt EWC} on 5 permuted Mnist sequence of tasks, hidden size=128, (b) hidden size=64. }
    \label{fig:SLNI_EWC}%
\end{figure}
\subsection{Cifar 100 sequence}
In section~\ref{sec:experiments:cifarimagenet} we have tested  \SLNI and other representation regularizers on the Cifar 100 sequence. In Figure~\ref{fig:cifarimagenet}(a) we compare their performance on a network with hidden layer size $256$. Figure~\ref{fig:cifar_128} 
%shows the test accuracy achieved by the compared methods on each task at the end of the sequence 
repeats the same experiment for a network with hidden size $128$.  While {\tt DeCov} and \SLNI continue to improve over {\tt No-Reg}, {\tt L1-Rep} seems to suffer in this case. Our interpretation is that {\tt L1-Rep} here interferes with the previously learned tasks while penalizing activations and hence suffers from catastophic forgetting. In line with all the previous experiments \SLNI achieves the best accuracies and manages here to improve over {$6\% $} compared to {\tt No-Reg}.
\begin{figure*}[h!]
\centering
\includegraphics[width=0.80\textwidth]{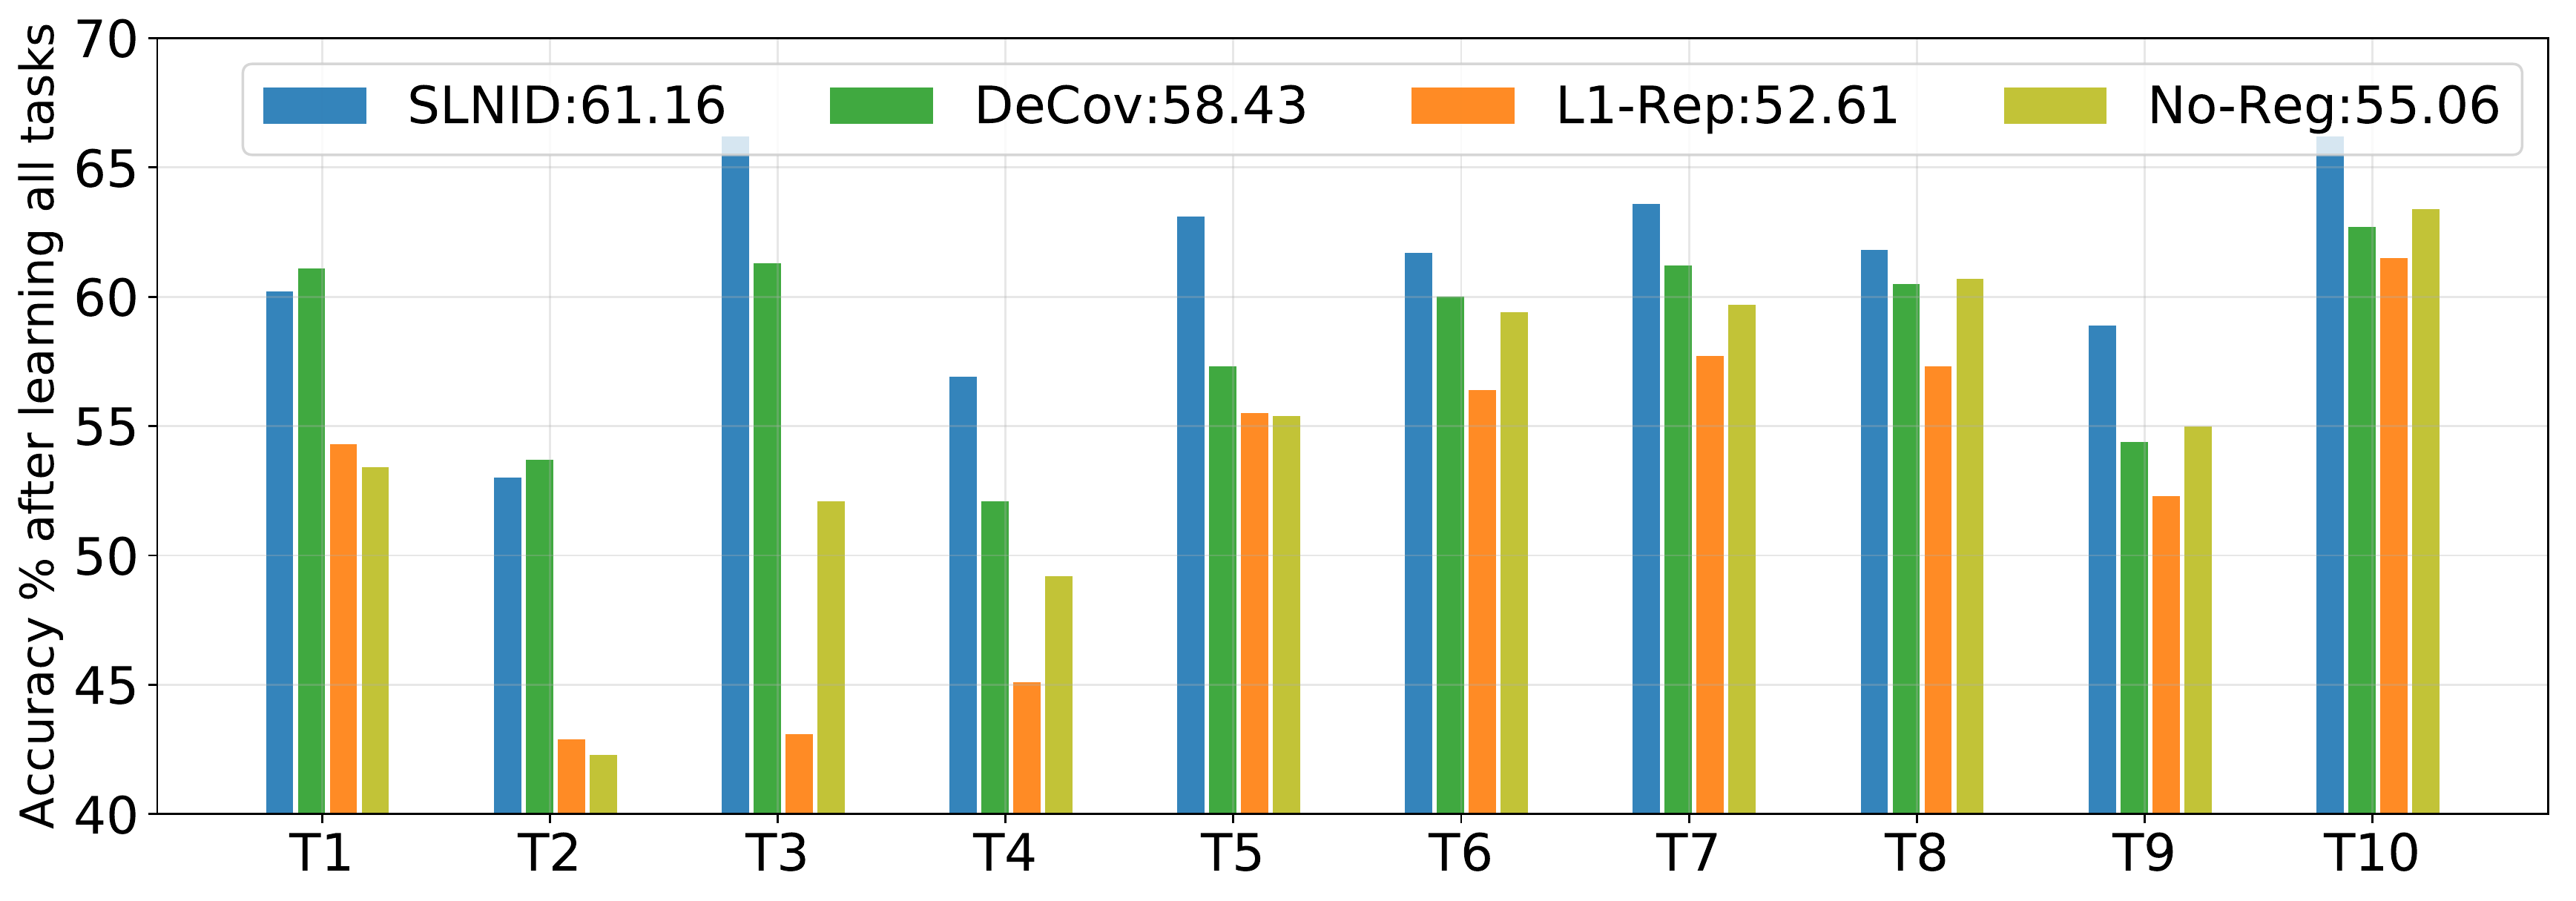} 
     \caption{\footnotesize  Comparison of different regularization techniques on a sequence of ten tasks from Cifar split. Hidden size=128. See Figure~\ref{fig:cifarimagenet}(a) for size 256.}%
    \label{fig:cifar_128}%
  
\end{figure*}

\subsection{Spatial Locality Test}
To avoid penalizing all the active neurons,  our \SLNI weights the correlation penalty between each two neurons based on their spatial distance using  a Gaussian function. We want to visualize the effect of this spatial locality on the neurons activity. To achieve this, we have used the first 3 tasks of the Permuted Mnist sequence as a test case and visualized the neurons importance after each task. This is done using the network of hidden layer size $64$. 
Figure~\ref{fig:scale1}, Figure~\ref{fig:scale2} and Figure~\ref{fig:scale3} show the neurons importance after each task. The left column is without locality, i.e. \SLNI, and the right column is \SLNI. Blue represents the first task, orange the second task and green the third task.
When using \SLNI, inhibition is applied in a local manner allowing more active neurons which could potentially improve the representation power. When learning the second task, new neurons become important regardless of their closeness to first task important neurons as those neurons are excluded from the inhibition. As such, new neurons are becoming active as new tasks are learned. For \SLNI all neural correlation is penalized in the first task. And for later tasks, very few neurons are able to become active and important for the new task due to the strong global inhibition, where previous neurons that are excluded from the inhibition are easier to be re-used.

% \newpage

% \begin{figure}[h]
% \vspace*{-0.2cm}
%     \centering
%     \subfloat{{\includegraphics[width=0.495\textwidth]{images/Scale_Test/activation00.pdf} }}%
%     \hfillx
%     \subfloat{{\includegraphics[width=0.495\textwidth]{images/Scale_Test/activation60.pdf} }}%
  
%     \caption{\footnotesize First layer neuron importance  after learning the first task. Left: SNI, Right: SLNI.  }
%     \label{fig:scale1}%
% \end{figure}
% %\todo{TT: Could you still add labels to the axes in those figures ?}
% \begin{figure}[h]
% \vspace*{-0.2cm}
%     \centering
%     \subfloat{{\includegraphics[width=0.495\textwidth]{images/Scale_Test/activation01.pdf} }}%
%     \hfillx
%     \subfloat{{\includegraphics[width=0.495\textwidth]{images/Scale_Test/activation61.pdf} }}%
  
%     \caption{\footnotesize First layer neuron importance after learning the second task. Left: SNI, Right: SLNI. }
%     \label{fig:scale2}%
% \end{figure}
% \begin{figure}[h]
% \vspace*{-0.2cm}
%     \centering
%     \subfloat{{\includegraphics[width=0.495\textwidth]{images/Scale_Test/activation02.pdf} }}%
%     \hfillx
%     \subfloat{{\includegraphics[width=0.495\textwidth]{images/Scale_Test/activation62.pdf} }}%
  
%     \caption{\footnotesize First layer neuron importance  after learning the third task. Left: SNI, Right: SLNI. }
%     \label{fig:scale3}%
% \end{figure}

\newpage
\begin{figure}[h]
\vspace*{-0.2cm}
    \centering
    \subfloat{{\includegraphics[width=0.495\textwidth]{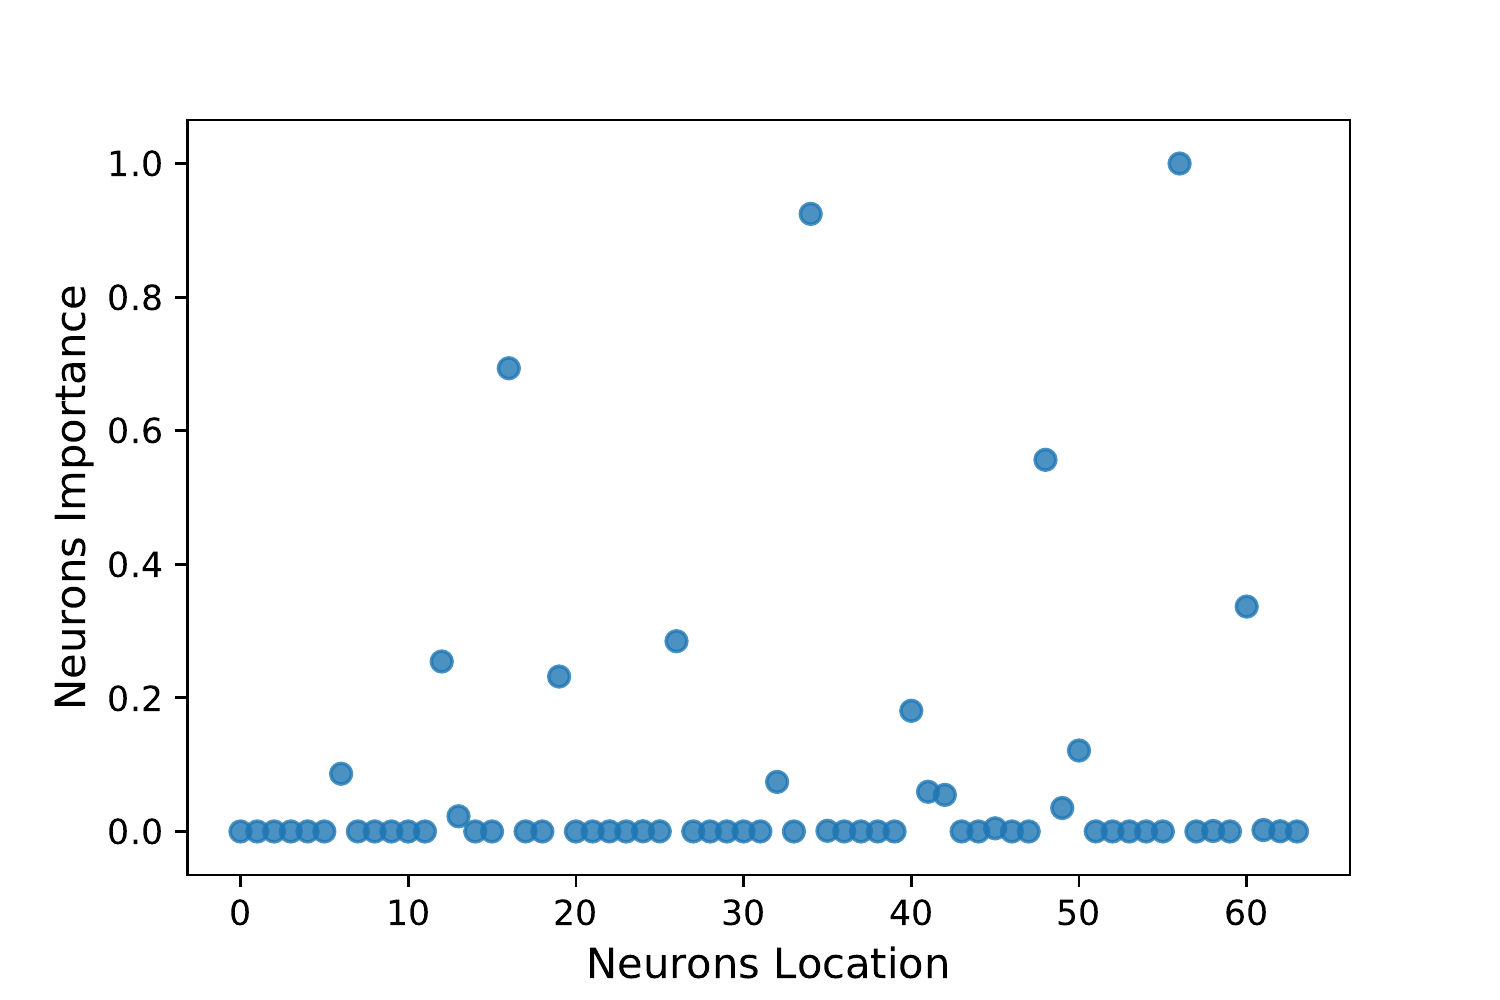} }}%
    \hfillx
    \subfloat{{\includegraphics[width=0.495\textwidth]{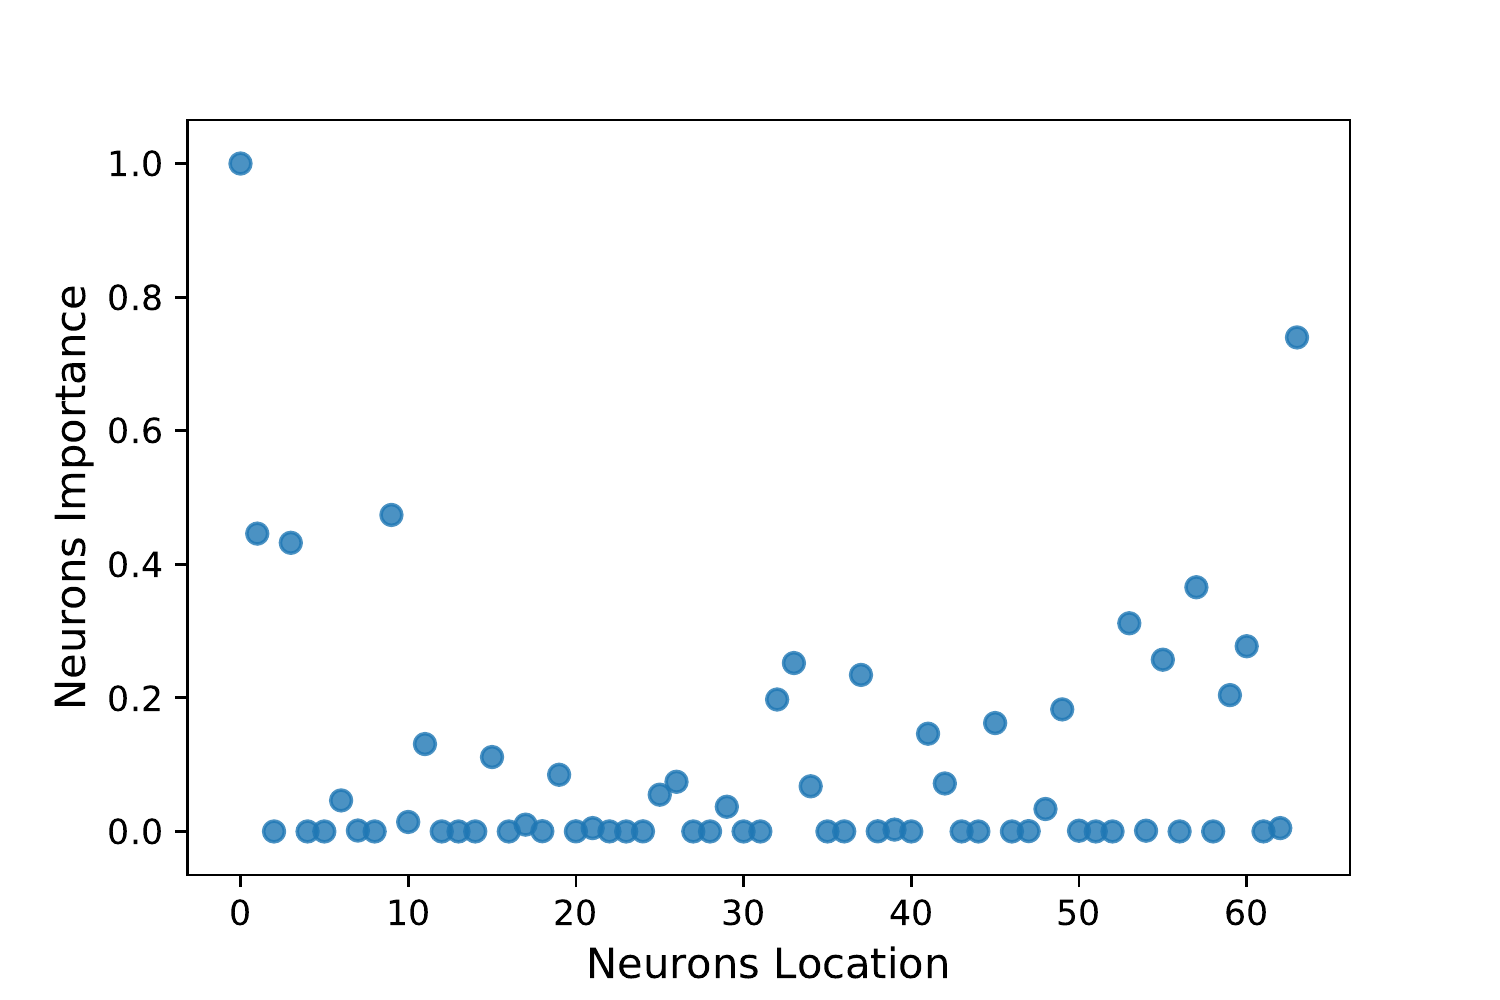} }}%
  
    \caption{\footnotesize First layer neuron importance after  learning the first task (blue). Left:  \SNI, Right:  \SLNI.  More active neurons are tolerated in  \SLNI.}
    \label{fig:scale1}%
\end{figure}

\begin{figure}[h]
\vspace*{-0.2cm}
    \centering
    \subfloat{{\includegraphics[width=0.495\textwidth]{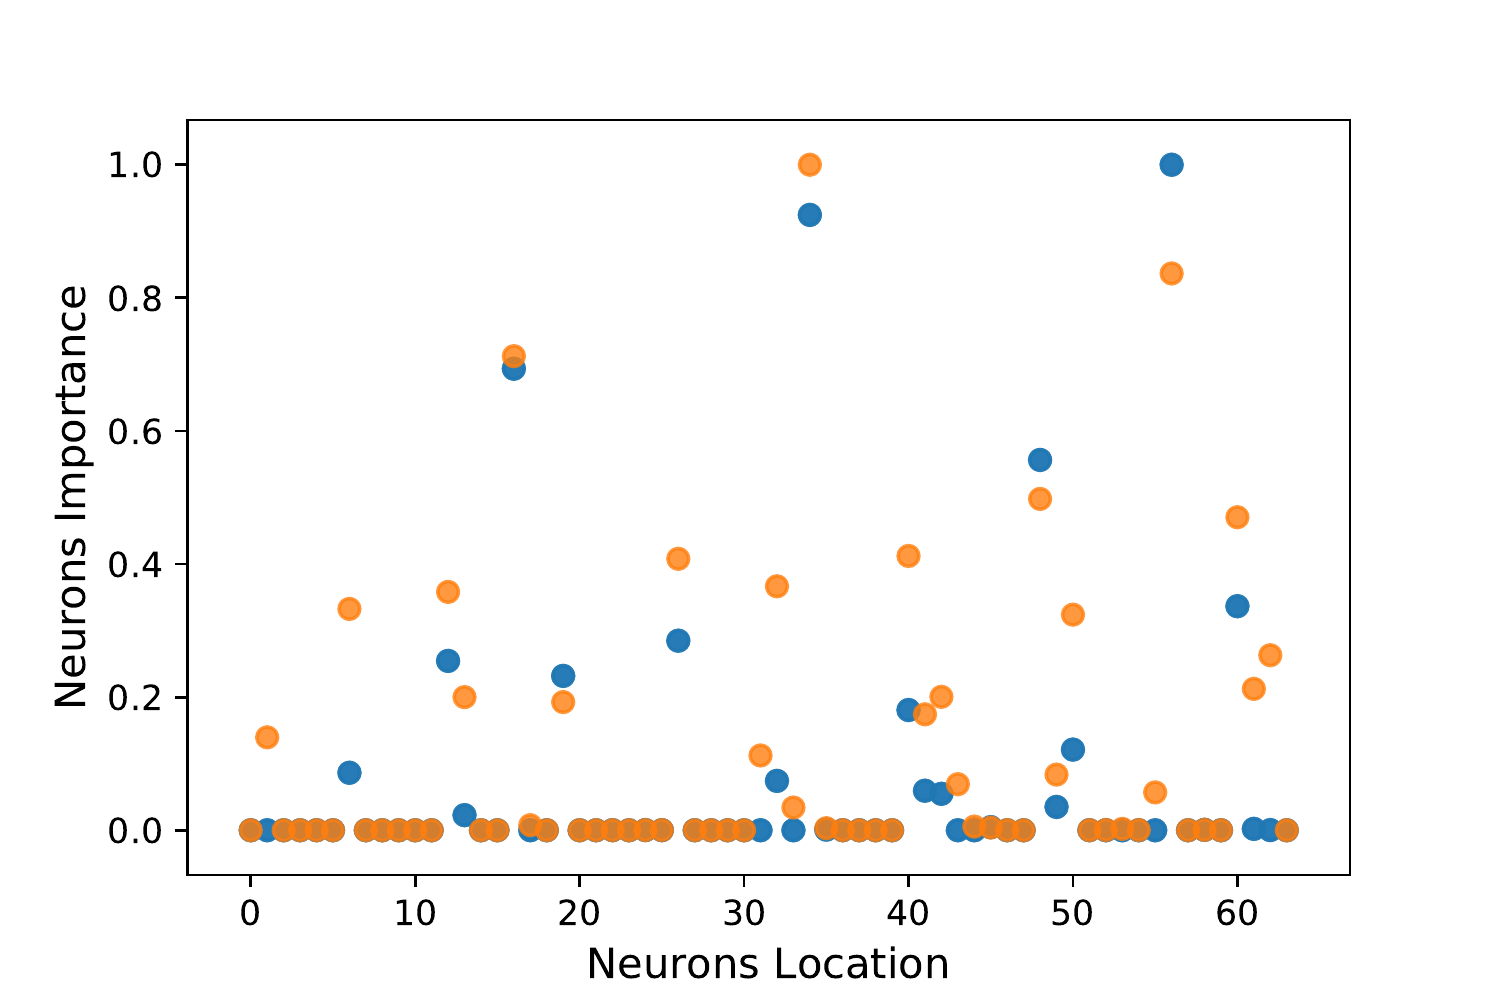} }}%
    \hfillx
    \subfloat{{\includegraphics[width=0.495\textwidth]{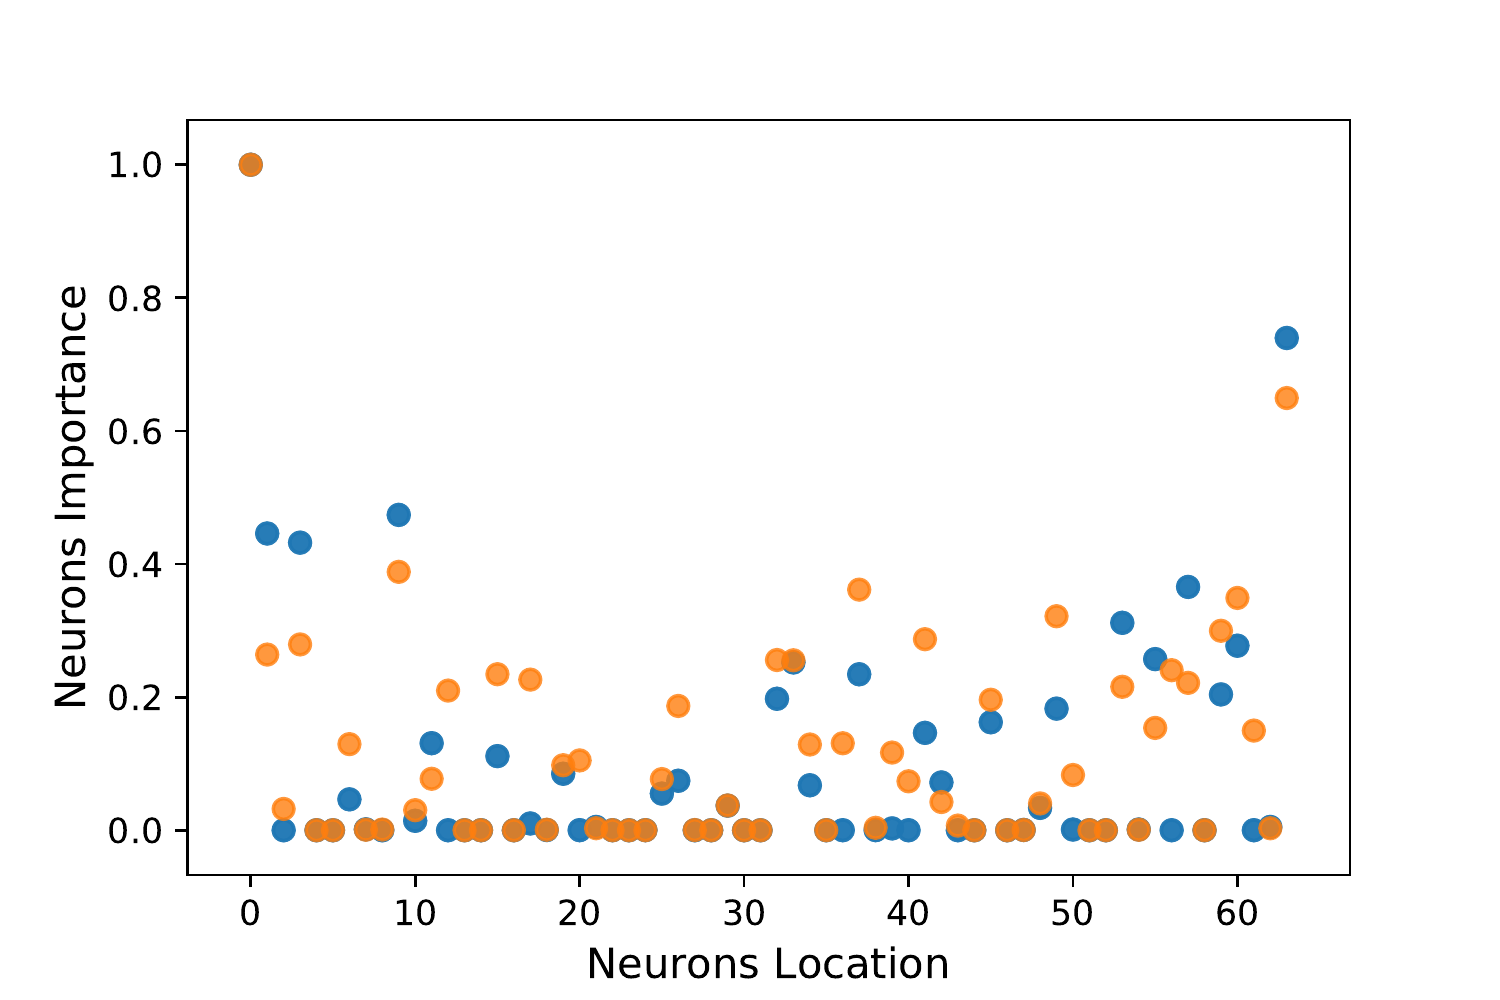} }}%
  
    \caption{\footnotesize First layer neuron importance  after learning the second task (orange), superimposed on Figure~\ref{fig:scale1}. Left: \SNI, Right: \SLNI. \SLNI allows new neurons, especially those that were close neighbours to previous important neurons, to become active and to be used for the new task. \SNI penalizes all unimportant neurons equally. As a result, previous neurons are adapted for the new tasks and less new neurons are getting activated. }
    \label{fig:scale2}%
\end{figure}
\begin{figure}[h]
\vspace*{-0.2cm}
    \centering
    \subfloat{{\includegraphics[width=0.495\textwidth]{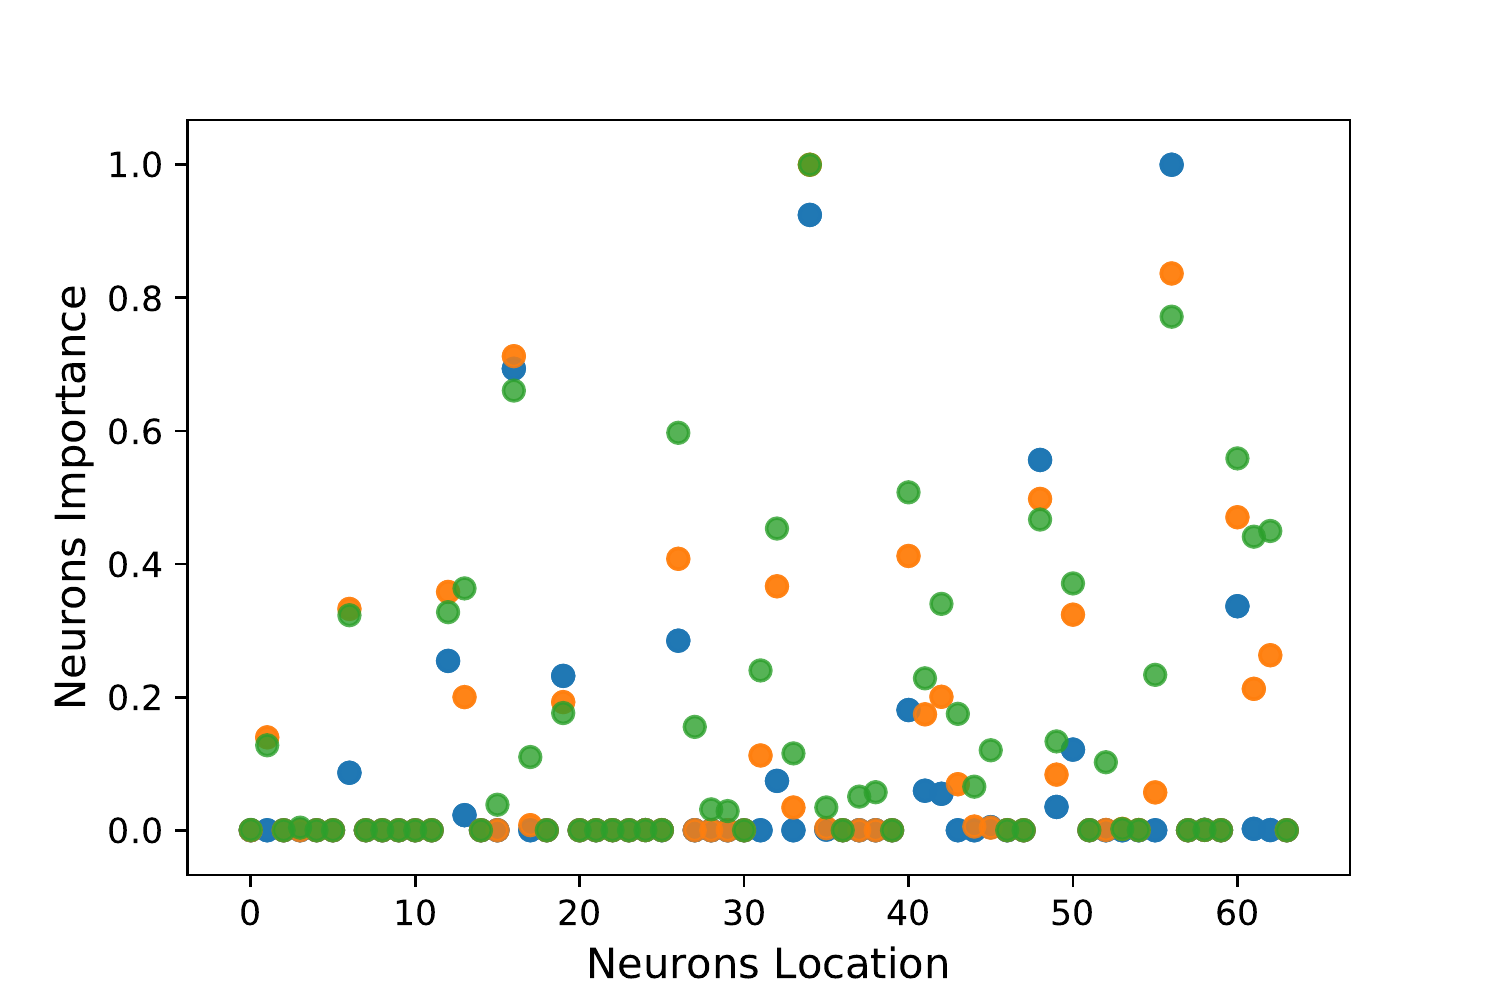} }}%
    \hfillx
    \subfloat{{\includegraphics[width=0.495\textwidth]{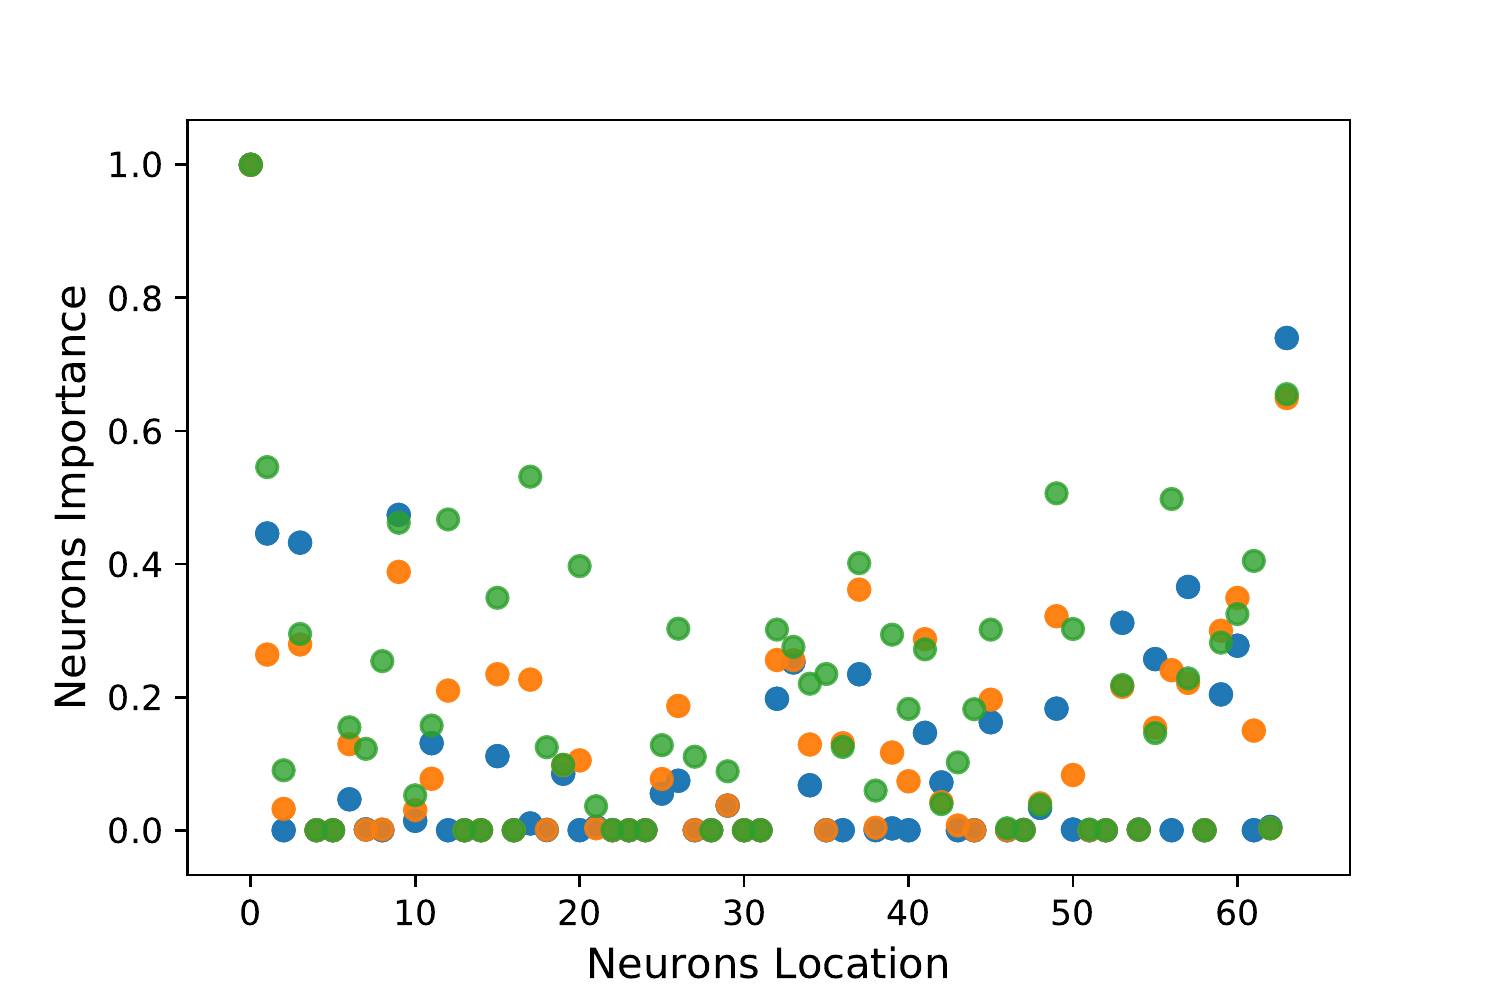} }}%
  
    \caption{\footnotesize First layer neuron importance after  learning the third task (green), superimposed on Figure~\ref{fig:scale2}. Left: \SNI, Right:  \SLNI.  \SLNI allows previous neurons to be re-used for the third task. It avoids changing the previous important neurons by adding new neurons. For \SNI, very few neurons are newly deployed. The new task is learned mostly by adapting previous important neurons, causing more interference. }
    \label{fig:scale3}%
\end{figure}
\newpage
\begin{figure}[h]
\vspace*{-0.2cm}
    \centering
    \subfloat{{\includegraphics[width=0.495\textwidth]{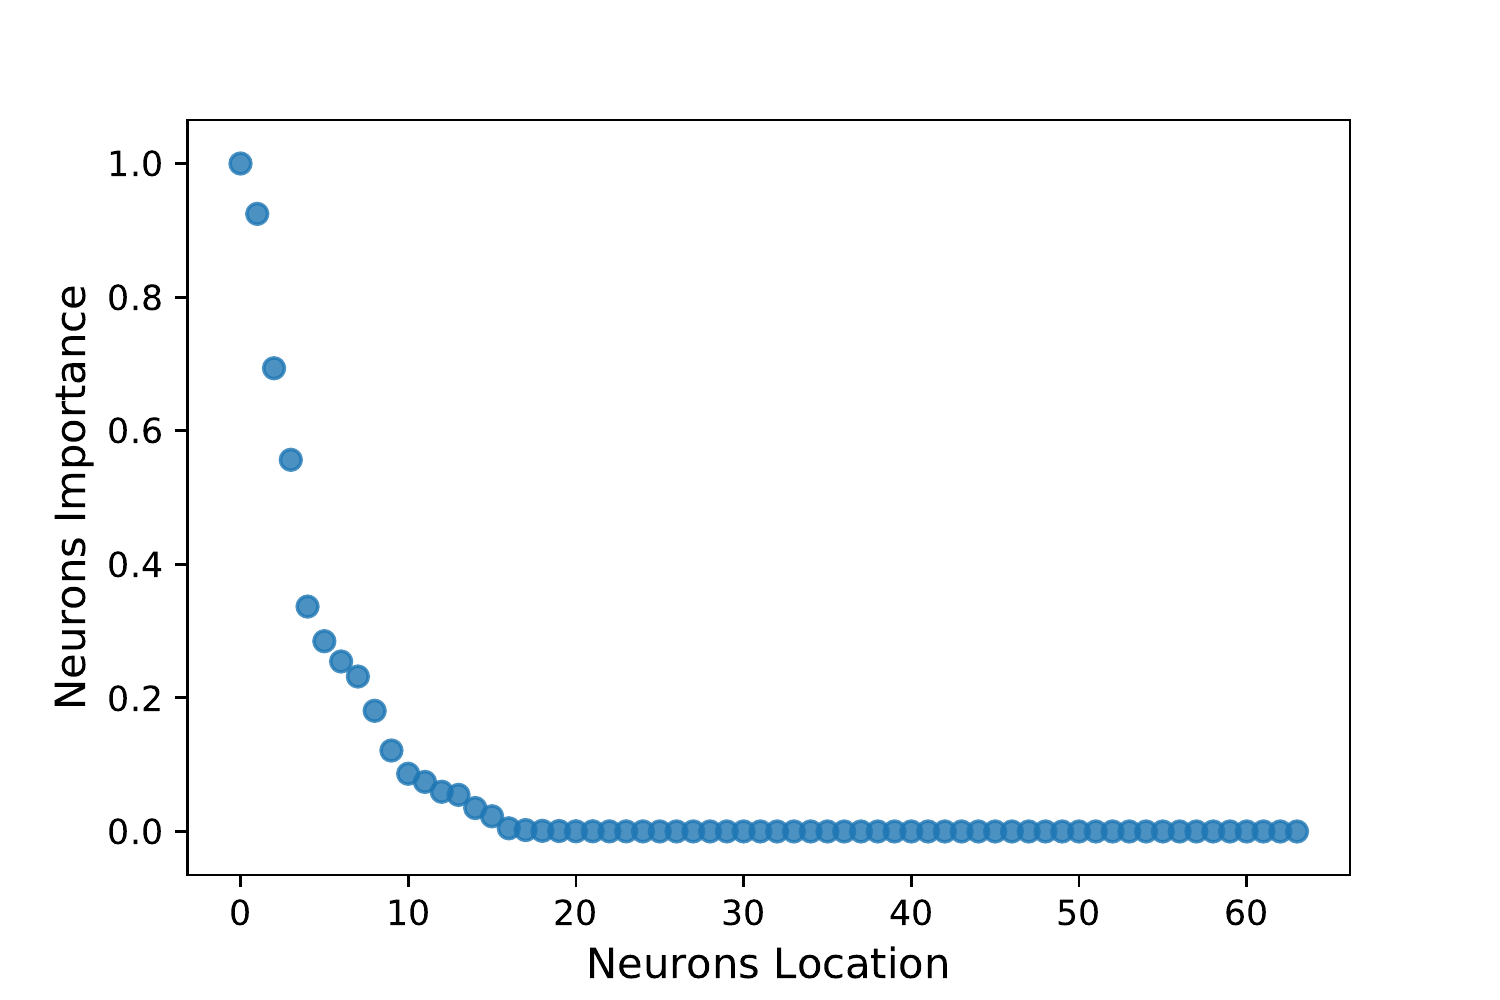} }}%
    \hfillx
    \subfloat{{\includegraphics[width=0.495\textwidth]{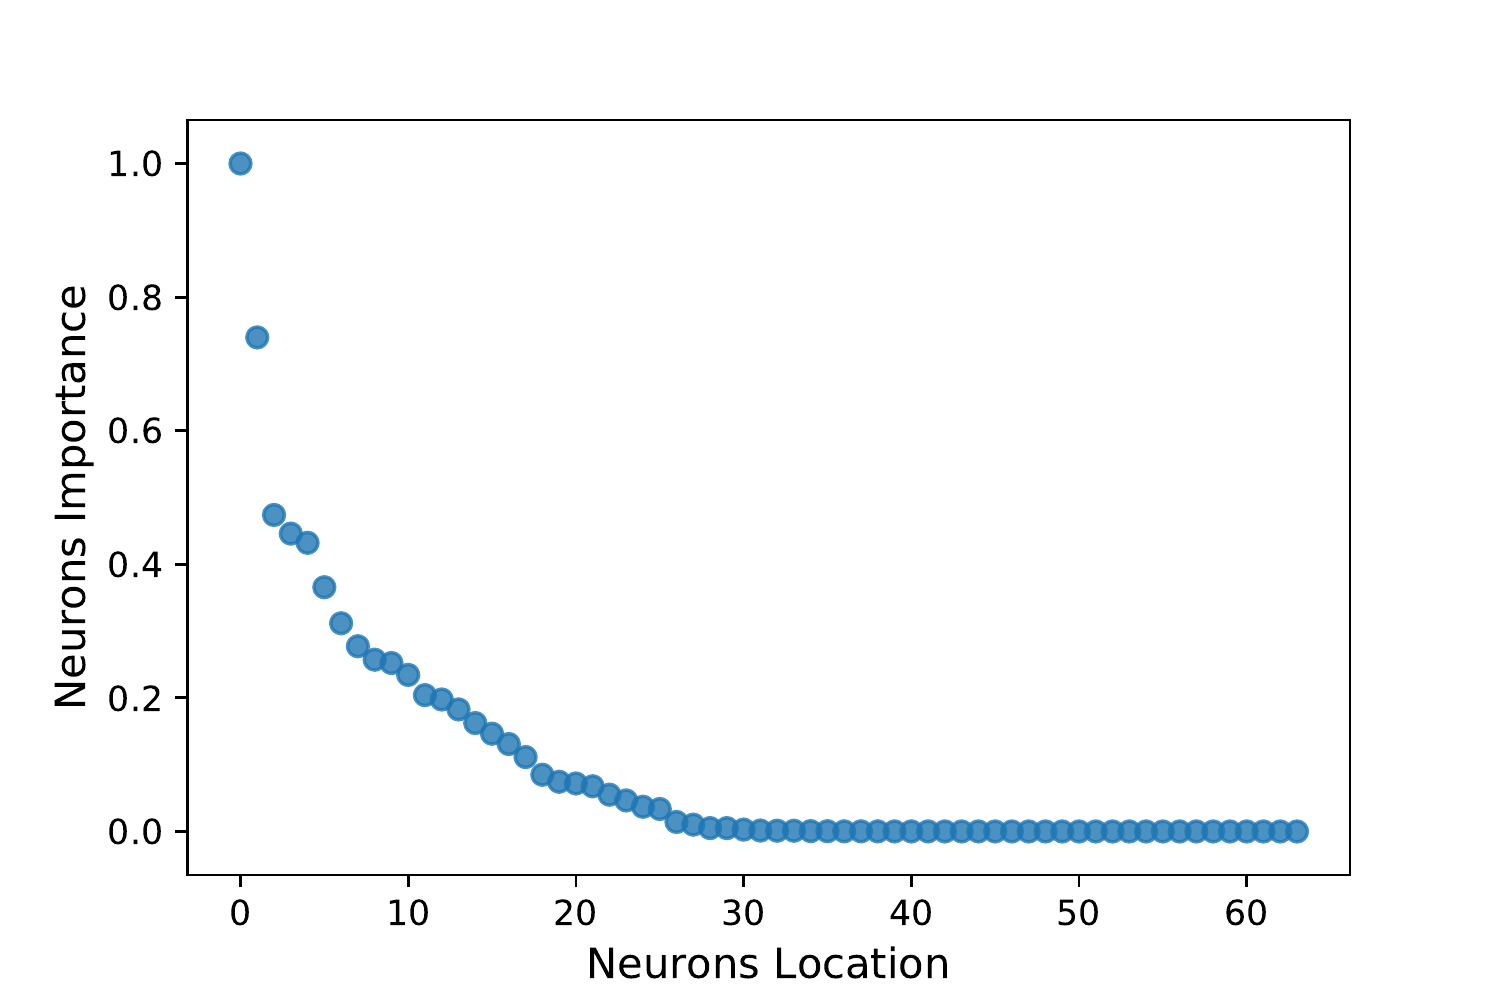} }}%
  
    \caption{\footnotesize First layer neuron importance after  learning the first task, sorted in descending order according to the first task neuron importance (blue). Left: \SNI, Right:  \SLNI.  More active neurons are tolerated in  \SLNI.}
    \label{fig:scale1b}%
\end{figure}
\begin{figure}[h]
\vspace*{-0.2cm}
    \centering
    \subfloat{{\includegraphics[width=0.495\textwidth]{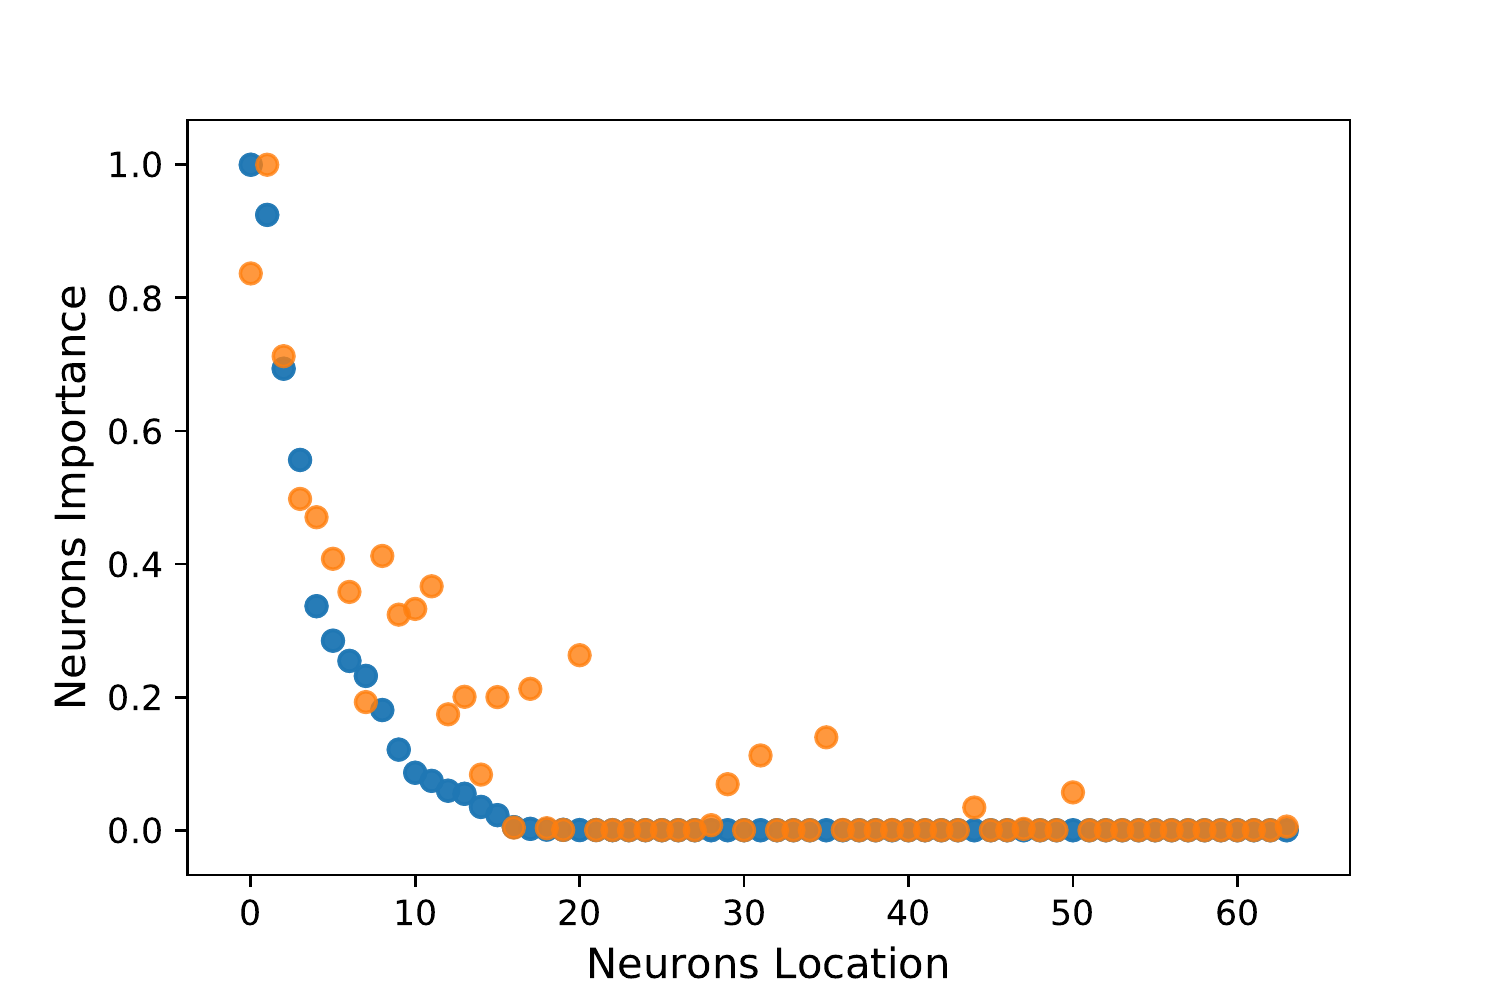} }}%
    \hfillx
    \subfloat{{\includegraphics[width=0.495\textwidth]{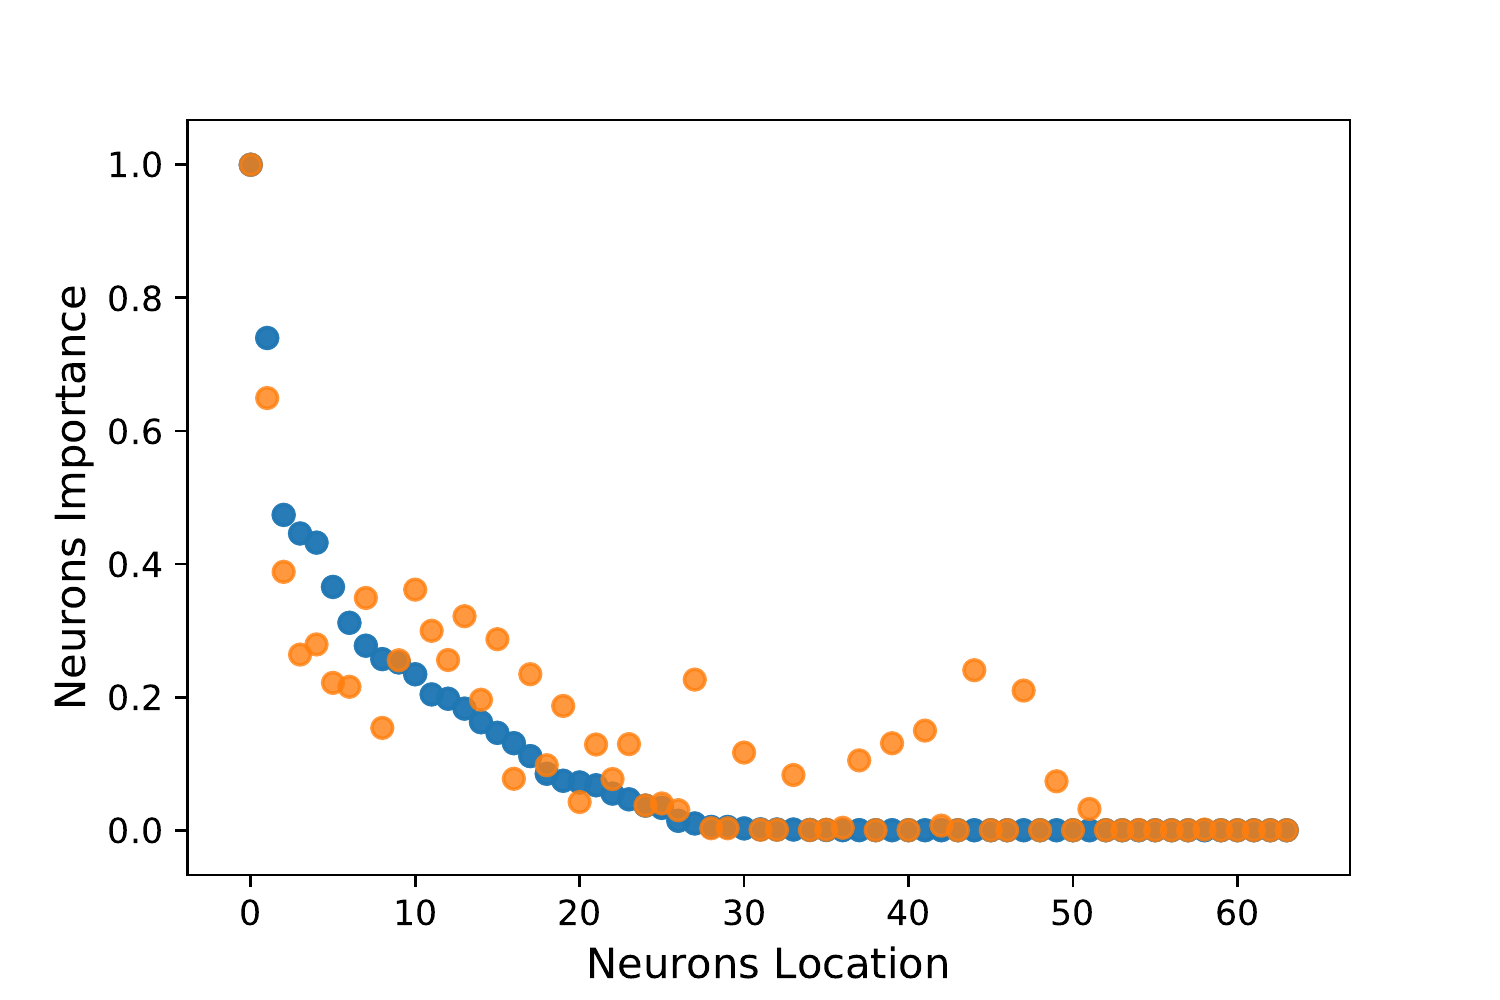} }}%
  
    \caption{\footnotesize First layer neuron importance  after learning the second task sorted in descending order according to the first task neuron importance (orange), superimposed on top of figure~\ref{fig:scale1b}. Left: \SNI, Right:  \SLNI.  \SLNI allows new neurons to become active and be used for the new task. \SNI penalizes all unimportant  neurons equally and hence more neurons are re-used then initiated for the first time. }
    \label{fig:scale2b}%
\end{figure}
\begin{figure}[h]
\vspace*{-0.4cm}
    \centering
    \subfloat{{\includegraphics[width=0.495\textwidth]{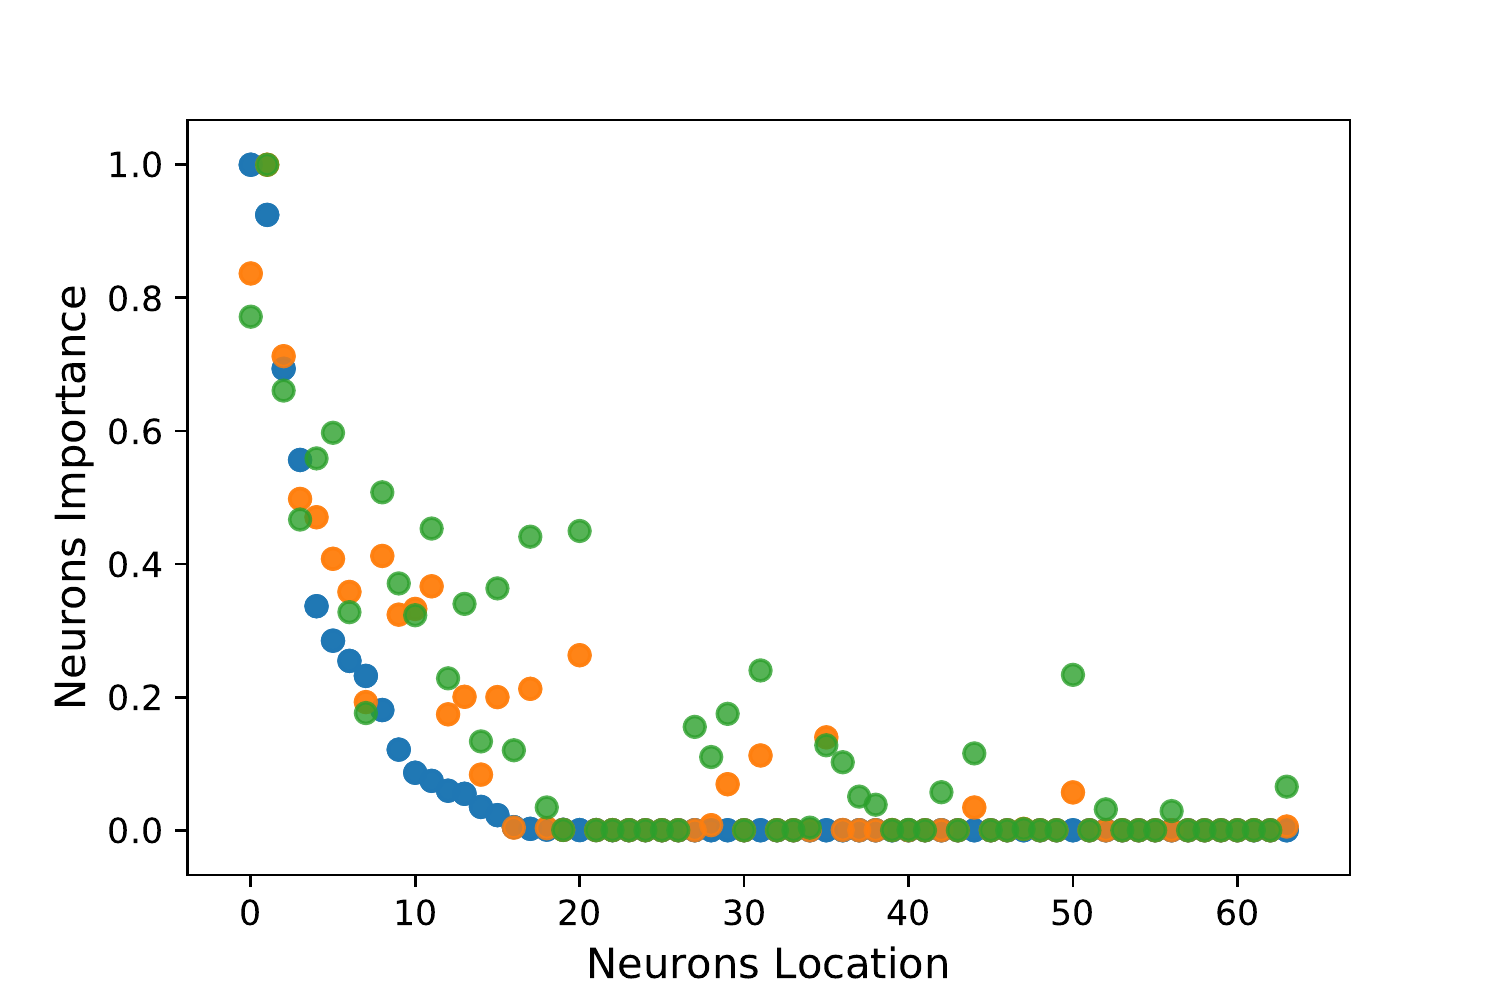} }}%
    \hfillx
    \subfloat{{\includegraphics[width=0.495\textwidth]{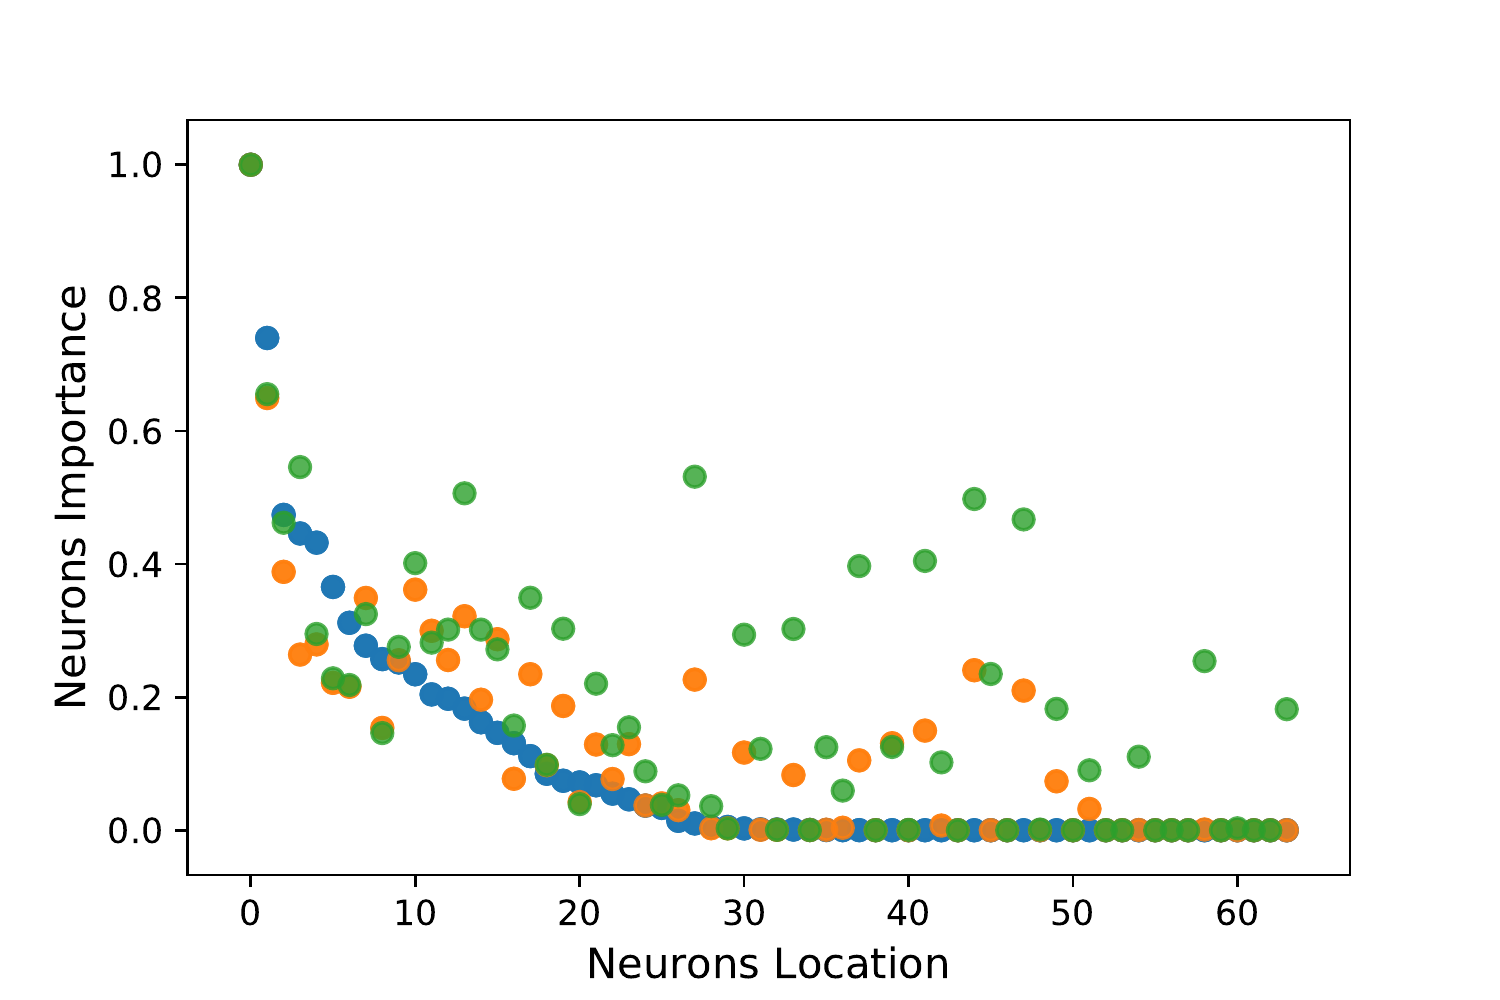} }}%
  
    \caption{\footnotesize First layer neuron importance after  learning the third task sorted in descending order according to the first task neuron importance (green), superimposed on top of figure~\ref{fig:scale2b}.  Left: \SNI, Right:  \SLNI.  \SLNI allows previous neurons to be re-used for the third task while activating new neurons to cope with the needs of the new task. For \SNI, very few neurons are newly deployed while most previous important neurons for previous tasks are re-adapted to learn the new task. }
    \label{fig:scale3b}%
\end{figure}
