# Supplementary material for: Continual Learning in Neural Networks
Source: arXiv:1910.02718 source file (2019-10-18)
Supplement: Supplementary file 2 [file myappendix.tex]

% !TeX root = ../../thesis.tex
\chapter{This is myappendix}\label{ch:myappendix}

\ldots

\instructionsappendices

%%%%%%%%%%%%%%%%%%%%%%%%%%%%%%%%%%%%%%%%%%%%%%%%%%
% Keep the following \cleardoublepage at the end of this file, 
% otherwise \includeonly includes empty pages.
\cleardoublepage

% vim: tw=70 nocindent expandtab foldmethod=marker foldmarker={{{}{,}{}}}
